# Supplementary material for: Unleashing the Power of Meta-tuning for Few-shot Generalization Through Sparse Interpolated Experts
Source: arXiv:2403.08477 source file (2024-07-01)
Supplement: Supplementary file 1 [file cl_with_smat.tex]

\subsection{Continual Learning with SMAT}
We show that SMAT could be even applied to continual learning scenarios, where the tasks are learned in a sequential manner. The goal of continual learning is to learn new unseen task fast while maintaining the performance of previous learned tasks. Here, we apply SMAT to two continual learning scenarios that involve meta-learning, including (i) conventional online learning setup and (ii) OSAKA~\citep{caccia2020online}, a realistic online learning setup, by applying sparse adaptation of SMAT to La-MAML~\citep{gupta2020look} and Continual-MAML~\citep{caccia2020online}, respectively.

\begin{table}[t]
\centering
  \caption{Retained accuracy (RA) and forward-transfer (FT) for three different MNIST continual learning problems: rotations, permutations and many permutations. Reported results are averaged over three trials, subscripts denote the standard deviation, and bold denotes the best result.}
  \small\centering
  \label{tab:mnist}
   \begin{tabular}{l ll ll ll}
    \toprule
    & \multicolumn{2}{c}{Rotations} & \multicolumn{2}{c}{Permutations} & \multicolumn{2}{c}{Many Permutations} \\
    \cmidrule(lr){2-3} \cmidrule(lr){4-5} \cmidrule(lr){6-7}
    & RA ($\uparrow$) & FT ($\uparrow$) & RA ($\uparrow$) & FT ($\uparrow$) & RA ($\uparrow$) & FT ($\uparrow$) \\
    \midrule
    C-MAML & 77.05\std{0.70} & 47.95\std{0.92} & 72.10\std{0.60}& -0.34\std{0.62} & 44.23\std{0.69}&  1.85\std{0.63} \\ 
    La-MAML & 76.57\std{0.79} & 47.87\std{0.98} & 73.66\std{0.46}& -0.19\std{0.55}  & 49.32\std{0.86}& 0.99\std{0.62} \\
    \textbf{+ SMAT (ours)} & \textbf{77.21\std{0.91}}& \textbf{50.36\std{0.88}} & \textbf{77.05\std{0.32}}& \textbf{-0.11\std{0.45}} & \textbf{51.66\std{0.60}}& \textbf{2.44\std{0.49}} \\ 
    \bottomrule
  \end{tabular}
\end{table}
\textbf{Conventional online learning.} Conventional online continual learning aims to train a model under the sequence of tasks by observing each task's training data sequentially.  Recently, several works in continual learning have highlighted the importance of forward transfer, i.e., leveraging the learned knowledge from the previous tasks to transfer and accelerate when learning new unseen tasks \citep{chen2023forgetting}. Here, we argue that SMAT can play a critical role to enhance forward transfer ability by combining with meta-continual learning approaches as our scheme is effective on learning unseen or out-of-distribution tasks.

To this end, we extend SMAT to continual learning setup by applying our sparse gradient adaptation algorithm to a recent meta-continual learning framework coined La-MAML~\citep{gupta2020look}. La-MAML mainly consists of three steps: (i) inner adaptation by minimizing the current task loss (ii) outer loss is calculated under the adapted model with the current task batch and the replay buffer that consists of past tasks to mitigate forgetting, and (iii) repopulating the replay buffer with the current task batch. Here, we extend SMAT for the inner adaptation to enhance the generalization on the unseen tasks by sparsifying the adaptation gradients. Note that we do not consider modulation for continual learning as we are using a small-sized model. Formally, for a given continual learner $\theta$ and tasks dataset $\mathcal{D}_t$, we sparsify the inner loop gradient with sparse binary mask $\mathbf{z}$ as follows:
%\begin{equation}
$\theta_{t} \leftarrow \theta - \max(0, \alpha) \circ \mathbf{z} \circ \nabla_{\theta}\mathcal{L}(\theta, \mathcal{D}_t)$
%\end{equation}
where $\alpha$ is the trainable element-wise learning rate (which is trained on the outer loop optimization) and $\max(\cdot,\cdot)$ selects the maximum value between the pairs. It is worth noting that using $\max(\cdot,\cdot)$ is originated from La-MAML which also induces gradient sparsity when the trained learning rate becomes negative value.

% We extend SMAT to La-MAML. La-MAML is this. 

We verify the efficacy of SMAT for continual learning under three different benchmarks including MNIST rotations, permutations, and many permutations where we utilize a single-headed network based by following the setup from \citep{gupta2020look}. Here, the network is not provided with task-specific information and each data sample is presented only once. We use the same hyper-parameters as in La-MAML, except for our additional sparsity regularization $\lambda$ and compare with C-MAML and La-MAML which are proposed in \citep{gupta2020look}.
As shown in Table \ref{tab:mnist}, using SMAT on La-MAML consistently and significantly outperforms the baselines in retain accuracy (i.e., average task accuracy at the final checkpoint) and forward transfer accuracy (i.e., accuracy improvement of future tasks over random initialization when learning the current task). For instance, using SMAT over the La-MAML improves more than 4.3\% retain accuracy in MNIST permutations. We find this improvement mainly comes from the forward transfer ability of SMAT, i.e., fast learning on new unseen tasks, which reflects that sparse gradient adaptation is indeed helpful for learning out-of-distribution domains and tasks. 

% (if possible, show sparsity pattern).

\begin{table*}[t]
\caption{Cumulative online accuracy (\%) on the Omniglot-MNIST-FashionMNIST online learning benchmark where tasks are switched with a probability of $1-p$. Reported results are averaged over five trials, subscripts denote the standard deviation, and bold denotes the best result of each group.}
\centering
\resizebox{\textwidth}{!}{
\begin{tabular}{lcccccccc}
    \toprule
    & \multicolumn{4}{c}{$p=0.98$} & \multicolumn{4}{c}{$p=0.90$} \\
    \cmidrule(lr){2-5} \cmidrule(lr){6-9}
    Method & Total & Omniglot & MNIST & Fashion & Total & Omniglot & MNIST & Fashion  \\ 
    \midrule
        Online ADAM & 73.9\std{2.2} & 81.7\std{2.3} & 70.0\std{3.6} & 62.3\std{2.5} & 23.8\std{1.2} & 26.6\std{2.0} & 20.0\std{1.4} & 22.1\std{1.3} \\
        Fine Tuning & 72.7\std{1.7} & 80.8\std{2.0} & 68.7\std{2.8} & 59.6\std{3.1} & 22.1\std{1.1} & 25.5\std{1.5} & 18.1\std{1.9} & 19.2\std{1.6} \\
        MAML & 84.5\std{1.7} & 97.3\std{0.3} & 80.4\std{0.3} & 63.5\std{0.3} & 75.5\std{0.7} & 88.8\std{0.4} & 68.1\std{0.5} & 56.2\std{0.4} \\
        ANIL & 75.3\std{2.0} & 95.1\std{0.6} & 58.7\std{2.9} & 49.7\std{0.3} & 69.1\std{0.8} & 88.3\std{0.5} & 52.4\std{0.6} & 47.6\std{0.9} \\
        BGD & 87.8\std{1.3} & 95.1\std{0.5} & 86.9\std{1.1} & 74.4\std{1.1} & 63.4\std{0.9} & 72.8\std{1.2} & 55.9\std{2.2} & 51.7\std{1.3} \\
        MetaCOG & 88.0\std{1.0} & 95.2\std{0.5} & 87.1\std{1.5} & 74.3\std{1.5} & 63.6\std{0.9} & 73.5\std{1.3} & 55.9\std{1.8} & 51.7\std{1.4} \\
        MetaBGD  & 91.1\std{2.6} & 96.8\std{1.5} & 92.5\std{1.9} & 77.8\std{3.8} & 74.8\std{1.1} & 83.1\std{1.0} & 71.7\std{1.5} & 61.5\std{1.2} \\
        Continual MAML  &  92.8\std{0.6} &  \textbf{97.8\std{0.2}} & 93.9\std{0.8} & 79.9\std{0.7} & 83.3\std{0.4} & 89.0\std{0.5} & 84.5\std{0.7} & 71.1\std{0.7} \\
        \textbf{+ SMAT (ours)} & \textbf{93.3\std{0.7}} & 97.5\std{0.4} & \textbf{94.4\std{0.7}} & \textbf{81.5\std{0.8}} & \textbf{85.5\std{0.7}} & \textbf{89.2\std{0.6}} & \textbf{86.4\std{0.8}} & \textbf{74.6\std{0.6}} \\
    \bottomrule
    \end{tabular}
  }
\label{tab:omniglot}
\end{table*}

\textbf{Realistic online learning.}
We also consider an additional continual learning scenario coined OSAKA~\citep{caccia2020online}, which evaluates the learner based on the randomly emerging tasks. To be specific, unlike conventional continual learning that measures the performance at the final checkpoint, OSAKA measures the cumulative adaptation accuracy at the current task $t$ where such a task is randomly chosen from past and future tasks of in-distribution domain and out-of-distribution domains as well. 

% To this end, we extend SMAT to continual learning setup by applying our sparse gradient adaptation algorithm to a recent meta-continual learning framework coined La-MAML~\citep{gupta2020look}.

In this setup, we extend Continual MAML~\citep{caccia2020online}, a recently proposed continual learning framework based on MAML~\citep{finn2017model} by utilizing our sparse gradient adaptation in the inner loop. In essence, Continual MAML augments the original MAML framework by integrating a task-switch detection mechanism predicated on fluctuations in loss. Data accumulates in a buffer until a task switch is identified. Upon detection, the buffered data facilitates a meta-parameter update, subsequently clearing the buffer and initiating a fresh inner-loop optimization. 

We validate the effectiveness of SMAT on Omniglot-MNIST-FashionMNIST online learning benchmark. We consider the following baselines from \citep{caccia2020online}, including, Online Adam, Fine Tuning, MAML~\citep{finn2017model}, ANIL~\citep{raghu2019rapid}, BGD~\citep{zeno2018task}, MetaCOG~\citep{he2019task}, MetaBGD~\citep{he2019task}, and Continaul MAML~\citep{caccia2020online}.
As presented in Table \ref{tab:omniglot}, SMAT outperforms the baseline in most of cases where it typically shows high improvement on out-of-distribution tasks, e.g., improvement of 3.5\% over Continual MAML in Fashion MNIST task under $p=0.90$. We remark that our major contribution is to enhance the generalization ability of adaptation by introducing sparse adaptation where this results re-emphasize the ability of SMAT (or sparse adaptation) on learning novel (or unseen) tasks.
