# Supplementary material for: Unleashing the Power of Meta-tuning for Few-shot Generalization Through Sparse Interpolated Experts
Source: arXiv:2403.08477 source file (2024-07-01)
Supplement: Supplementary file 2 [file continual_learning_setup.tex]

% \section{Experimental details of continual learning}

% \textbf{Baselines.}

% \textbf{Training details.}

% \textbf{Evaluation details.}
